# Supplementary material for: A 3.3 Gbps SPAD-Based Quantum Random Number Generator
Source: arXiv:2209.04868 source file (2022-09-11)
Supplement: Supplementary file 1 [file sec11_appendix1.tex]

\appendix[Derivation of QRFF Bias Model]\label{appendix1}
\begin{gather*}
t_1 = (i-\eta)(t_r - t_f) + t_h, \\ 
t_0 = \eta(t_r+t_f) + t_l \\
t_0 + t_1 = \dfrac{2}{\lambda_D} \\
t_h = \dfrac{1}{\lambda_D} - t_r \\
t_l = \dfrac{1}{\lambda_D} - t_f \\
\end{gather*}

\begin{align}
P_1 &= \dfrac{t_1}{t_1+t_0} \nonumber\\
&= \dfrac{(1-\eta)(t_r+t_f) + \lambda_D -t_r}{2\lambda_D} \nonumber\\
&= \dfrac{\lambda_D}{2\lambda_D} + \dfrac{t_f-\eta(t_r+t_f)}{2}\cdot\lambda_D \nonumber\\
&= \dfrac{1}{2} + \dfrac{t_f-\eta(t_r+t_f)}{2}\cdot\lambda_D
\end{align}

\begin{align}
b = \dfrac{t_f-\eta(t_r+t_f)}{2}\cdot\lambda_D
\end{align}
